# Supplementary material for: County-level Algorithmic Audit of Racial Bias in Twitter's Home Timeline
Source: arXiv:2211.08667 source file (2023-02-10)
Supplement: Supplementary file 1 [file 04_appendix.tex]

\section{List of US counties with missing data} \label{appendix:missing}

\begin{longtable}{llll}

\caption{List of counties with no users assigned to them\label{table:missing}}\\
 \hline
  County id & Name & State & Population\\
 \hline
 \endfirsthead
28055     &            Issaquena County &   Mississippi &              1328 \\
21201     &            Robertson County &      Kentucky &              2143 \\
31113     &                Logan County &      Nebraska &               886 \\
72121     &  Sabana Grande Municipality &   Puerto Rico &             23054 \\
72067     &    Hormigueros Municipality &   Puerto Rico &             16180 \\
72015     &         Arroyo Municipality &   Puerto Rico &             18111 \\
72137     &       Toa Baja Municipality &   Puerto Rico &             79726 \\
51775     &                       Salem &      Virginia &             25519 \\
51530     &                 Buena Vista &      Virginia &              6399 \\
51790     &                    Staunton &      Virginia &             24452 \\
51678     &                   Lexington &      Virginia &              7110 \\
51570     &            Colonial Heights &      Virginia &             17593 \\
51720     &                      Norton &      Virginia &              3990 \\
30069     &            Petroleum County &       Montana &               432 \\
51595     &                     Emporia &      Virginia &              5381 \\
46063     &              Harding County &  South Dakota &              1311 \\
8053      &             Hinsdale County &      Colorado &               878 \\
72103     &        Naguabo Municipality &   Puerto Rico &             26266 \\
51690     &                Martinsville &      Virginia &             13101 \\
72087     &          Loíza Municipality &   Puerto Rico &             26463 \\
72031     &       Carolina Municipality &   Puerto Rico &            157453 \\
72089     &       Luquillo Municipality &   Puerto Rico &             18547 \\
51081     &          Greensville County &      Virginia &             11659 \\
72139     &  Trujillo Alto Municipality &   Puerto Rico &             67780 \\
72061     &       Guaynabo Municipality &   Puerto Rico &             88663 \\
72021     &        Bayamón Municipality &   Puerto Rico &            182955 \\
72051     &         Dorado Municipality &   Puerto Rico &             37208 \\
72025     &         Caguas Municipality &   Puerto Rico &            131363 \\
72077     &         Juncos Municipality &   Puerto Rico &             39128 \\
72091     &         Manatí Municipality &   Puerto Rico &             39692 \\
72053     &        Fajardo Municipality &   Puerto Rico &             32001 \\
72127     &       San Juan Municipality &   Puerto Rico &            344606 \\
31007     &               Banner County &      Nebraska &               696 \\
72057     &        Guayama Municipality &   Puerto Rico &             41706 \\
13101     &               Echols County &       Georgia &              3994 \\
72147     &        Vieques Municipality &   Puerto Rico &              8771 \\
51600     &                     Fairfax &      Virginia &             23865 \\
72095     &        Maunabo Municipality &   Puerto Rico &             11023 \\
51580     &                   Covington &      Virginia &              5582 \\
13289     &               Twiggs County &       Georgia &              8284 \\
51840     &                  Winchester &      Virginia &             27789 \\
72007     &   Aguas Buenas Municipality &   Puerto Rico &             26275 \\
72043     &          Coamo Municipality &   Puerto Rico &             39265 \\
72047     &        Corozal Municipality &   Puerto Rico &             34165 \\
51540     &             Charlottesville &      Virginia &             47042 \\
72041     &          Cidra Municipality &   Puerto Rico &             40343 \\
72055     &        Guánica Municipality &   Puerto Rico &             16783 \\
72083     &     Las Marías Municipality &   Puerto Rico &              8599 \\
72029     &      Canóvanas Municipality &   Puerto Rico &             46108 \\
72027     &          Camuy Municipality &   Puerto Rico &             32222 \\
72145     &      Vega Baja Municipality &   Puerto Rico &             53371 \\
51660     &                Harrisonburg &      Virginia &             53391 \\
72013     &        Arecibo Municipality &   Puerto Rico &             87242 \\
72033     &         Cataño Municipality &   Puerto Rico &             24888 \\
72063     &         Gurabo Municipality &   Puerto Rico &             46894 \\
72069     &        Humacao Municipality &   Puerto Rico &             53466 \\
51685     &               Manassas Park &      Virginia &             16423 \\
72101     &        Morovis Municipality &   Puerto Rico &             31320 \\
72045     &        Comerío Municipality &   Puerto Rico &             19539 \\
72019     &   Barranquitas Municipality &   Puerto Rico &             28755 \\
8057      &              Jackson County &      Colorado &              1296 \\
72001     &       Adjuntas Municipality &   Puerto Rico &             18181 \\
72039     &         Ciales Municipality &   Puerto Rico &             16912 \\
72079     &          Lajas Municipality &   Puerto Rico &             23315 \\
72129     &    San Lorenzo Municipality &   Puerto Rico &             37873 \\
72151     &        Yabucoa Municipality &   Puerto Rico &             34149 \\
72011     &         Añasco Municipality &   Puerto Rico &             27368 \\
72085     &    Las Piedras Municipality &   Puerto Rico &             37768 \\
72113     &          Ponce Municipality &   Puerto Rico &            143926 \\
48261     &               Kenedy County &         Texas &               595 \\
72135     &       Toa Alta Municipality &   Puerto Rico &             73405 \\
72097     &       Mayagüez Municipality &   Puerto Rico &             77255 \\
72054     &        Florida Municipality &   Puerto Rico &             11910 \\
51750     &                     Radford &      Virginia &             17630 \\
72037     &          Ceiba Municipality &   Puerto Rico &             11853 \\
72143     &      Vega Alta Municipality &   Puerto Rico &             37724 \\
13239     &              Quitman County &       Georgia &              2276 \\
72017     &    Barceloneta Municipality &   Puerto Rico &             24299 \\
21091     &              Hancock County &      Kentucky &              8719 \\
48033     &               Borden County &         Texas &               665 \\
72049     &        Culebra Municipality &   Puerto Rico &              1314 \\
55078     &            Menominee County &     Wisconsin &              4579 \\
72073     &         Jayuya Municipality &   Puerto Rico &             14906 \\
72093     &        Maricao Municipality &   Puerto Rico &              6202 \\
72081     &          Lares Municipality &   Puerto Rico &             26451 \\
72105     &      Naranjito Municipality &   Puerto Rico &             28557 \\
72109     &       Patillas Municipality &   Puerto Rico &             17334 \\
72003     &         Aguada Municipality &   Puerto Rico &             38643 \\
72099     &           Moca Municipality &   Puerto Rico &             36872 \\
72071     &        Isabela Municipality &   Puerto Rico &             42420 \\
72125     &     San Germán Municipality &   Puerto Rico &             32114 \\
72149     &       Villalba Municipality &   Puerto Rico &             22993 \\
51820     &                  Waynesboro &      Virginia &             21926 \\
72005     &      Aguadilla Municipality &   Puerto Rico &             54166 \\
72131     &  San Sebastián Municipality &   Puerto Rico &             37964 \\
72111     &       Peñuelas Municipality &   Puerto Rico &             20984 \\
72141     &         Utuado Municipality &   Puerto Rico &             29402 \\
72133     &   Santa Isabel Municipality &   Puerto Rico &             22066 \\
72123     &        Salinas Municipality &   Puerto Rico &             28633 \\
72119     &     Río Grande Municipality &   Puerto Rico &             50550 \\
72115     &   Quebradillas Municipality &   Puerto Rico &             24036 \\
13307     &              Webster County &       Georgia &              2613 \\
72065     &        Hatillo Municipality &   Puerto Rico &             40390 \\
72153     &          Yauco Municipality &   Puerto Rico &             36439 \\
72117     &         Rincón Municipality &   Puerto Rico &             14269 \\
72035     &          Cayey Municipality &   Puerto Rico &             44530 \\
51770     &                     Roanoke &      Virginia &             99621 \\
72009     &       Aibonito Municipality &   Puerto Rico &             23457 \\
72059     &     Guayanilla Municipality &   Puerto Rico &             19008 \\
72075     &     Juana Díaz Municipality &   Puerto Rico &             46960 \\
72023     &      Cabo Rojo Municipality &   Puerto Rico &             49005 \\
55037     &             Florence County &     Wisconsin &              4337 \\
15005     &              Kalawao County &        Hawaii &                75 \\
38087     &                Slope County &  North Dakota &               704 \\
72107     &       Orocovis Municipality &   Puerto Rico &             21407 \\
51683     &                    Manassas &      Virginia &             41457 \\
2275      &                    Wrangell &        Alaska &              2484 \\
48269     &                 King County &         Texas &               228 \\
48155     &                Foard County &         Texas &              1408 \\
28039     &               George County &   Mississippi &             23710 \\

 \end{longtable}
