# Supplementary material for: County-level Algorithmic Audit of Racial Bias in Twitter's Home Timeline
Source: arXiv:2211.08667 source file (2023-02-10)
Supplement: Supplementary file 2 [file appendix_internal.tex]

\subsection{Appendix}
\subsubsection{black, weighted}
\begin{center}
\begin{tabular}{lclc}
\toprule
\textbf{Dep. Variable:}    &  promoted\_perc  & \textbf{  R-squared:         } &      0.007    \\
\textbf{Model:}            &       WLS        & \textbf{  Adj. R-squared:    } &      0.006    \\
\textbf{Method:}           &  Least Squares   & \textbf{  F-statistic:       } &      20.48    \\
\textbf{Date:}             & Tue, 25 Jan 2022 & \textbf{  Prob (F-statistic):} &   6.25e-06    \\
\textbf{Time:}             &     02:33:02     & \textbf{  Log-Likelihood:    } &    -703.67    \\
\textbf{No. Observations:} &        3072      & \textbf{  AIC:               } &      1411.    \\
\textbf{Df Residuals:}     &        3070      & \textbf{  BIC:               } &      1423.    \\
\textbf{Df Model:}         &           1      & \textbf{                     } &               \\
\bottomrule
\end{tabular}
\begin{tabular}{lcccccc}
                     & \textbf{coef} & \textbf{std err} & \textbf{t} & \textbf{P$> |$t$|$} & \textbf{[0.025} & \textbf{0.975]}  \\
\midrule
\textbf{const}       &       0.4923  &        0.002     &   241.913  &         0.000        &        0.488    &        0.496     \\
\textbf{black\_perc} &       0.0490  &        0.011     &     4.526  &         0.000        &        0.028    &        0.070     \\
\bottomrule
\end{tabular}
\begin{tabular}{lclc}
\textbf{Omnibus:}       & 2711.791 & \textbf{  Durbin-Watson:     } &      1.995    \\
\textbf{Prob(Omnibus):} &   0.000  & \textbf{  Jarque-Bera (JB):  } & 12894942.443  \\
\textbf{Skew:}          &  -2.649  & \textbf{  Prob(JB):          } &       0.00    \\
\textbf{Kurtosis:}      & 320.354  & \textbf{  Cond. No.          } &       8.39    \\
\bottomrule
\end{tabular}
%\caption{WLS Regression Results}
\end{center}

\subsubsection{black, unweighted}
\begin{center}
\begin{tabular}{lclc}
\toprule
\textbf{Dep. Variable:}    &  promoted\_perc  & \textbf{  R-squared:         } &     0.014   \\
\textbf{Model:}            &       OLS        & \textbf{  Adj. R-squared:    } &     0.014   \\
\textbf{Method:}           &  Least Squares   & \textbf{  F-statistic:       } &     44.94   \\
\textbf{Date:}             & Tue, 25 Jan 2022 & \textbf{  Prob (F-statistic):} &  2.41e-11   \\
\textbf{Time:}             &     02:33:02     & \textbf{  Log-Likelihood:    } &    2838.6   \\
\textbf{No. Observations:} &        3072      & \textbf{  AIC:               } &    -5673.   \\
\textbf{Df Residuals:}     &        3070      & \textbf{  BIC:               } &    -5661.   \\
\textbf{Df Model:}         &           1      & \textbf{                     } &             \\
\bottomrule
\end{tabular}
\begin{tabular}{lcccccc}
                     & \textbf{coef} & \textbf{std err} & \textbf{t} & \textbf{P$> |$t$|$} & \textbf{[0.025} & \textbf{0.975]}  \\
\midrule
\textbf{Intercept}   &       0.5168  &        0.009     &    57.201  &         0.000        &        0.499    &        0.535     \\
\textbf{white\_perc} &      -0.0712  &        0.011     &    -6.704  &         0.000        &       -0.092    &       -0.050     \\
\bottomrule
\end{tabular}
\begin{tabular}{lclc}
\textbf{Omnibus:}       & 493.539 & \textbf{  Durbin-Watson:     } &    1.881  \\
\textbf{Prob(Omnibus):} &   0.000 & \textbf{  Jarque-Bera (JB):  } & 8149.340  \\
\textbf{Skew:}          &  -0.183 & \textbf{  Prob(JB):          } &     0.00  \\
\textbf{Kurtosis:}      &  10.971 & \textbf{  Cond. No.          } &     10.5  \\
\bottomrule
\end{tabular}
%\caption{OLS Regression Results}
\end{center}

\subsubsection{white, weighted}
\begin{center}
\begin{tabular}{lclc}
\toprule
\textbf{Dep. Variable:}    &  promoted\_perc  & \textbf{  R-squared:         } &      0.094    \\
\textbf{Model:}            &       WLS        & \textbf{  Adj. R-squared:    } &      0.093    \\
\textbf{Method:}           &  Least Squares   & \textbf{  F-statistic:       } &      316.9    \\
\textbf{Date:}             & Tue, 25 Jan 2022 & \textbf{  Prob (F-statistic):} &   1.53e-67    \\
\textbf{Time:}             &     02:33:02     & \textbf{  Log-Likelihood:    } &    -563.00    \\
\textbf{No. Observations:} &        3072      & \textbf{  AIC:               } &      1130.    \\
\textbf{Df Residuals:}     &        3070      & \textbf{  BIC:               } &      1142.    \\
\textbf{Df Model:}         &           1      & \textbf{                     } &               \\
\bottomrule
\end{tabular}
\begin{tabular}{lcccccc}
                     & \textbf{coef} & \textbf{std err} & \textbf{t} & \textbf{P$> |$t$|$} & \textbf{[0.025} & \textbf{0.975]}  \\
\midrule
\textbf{const}       &       0.5946  &        0.005     &   108.164  &         0.000        &        0.584    &        0.605     \\
\textbf{white\_perc} &      -0.1459  &        0.008     &   -17.801  &         0.000        &       -0.162    &       -0.130     \\
\bottomrule
\end{tabular}
\begin{tabular}{lclc}
\textbf{Omnibus:}       & 3471.774 & \textbf{  Durbin-Watson:     } &      2.042    \\
\textbf{Prob(Omnibus):} &   0.000  & \textbf{  Jarque-Bera (JB):  } & 10563802.773  \\
\textbf{Skew:}          &  -4.542  & \textbf{  Prob(JB):          } &       0.00    \\
\textbf{Kurtosis:}      & 290.136  & \textbf{  Cond. No.          } &       9.35    \\
\bottomrule
\end{tabular}
%\caption{WLS Regression Results}
\end{center}

\subsubsection{white, unweighted}
\begin{center}
\begin{tabular}{lclc}
\toprule
\textbf{Dep. Variable:}    &  promoted\_perc  & \textbf{  R-squared:         } &     0.014   \\
\textbf{Model:}            &       OLS        & \textbf{  Adj. R-squared:    } &     0.014   \\
\textbf{Method:}           &  Least Squares   & \textbf{  F-statistic:       } &     44.94   \\
\textbf{Date:}             & Tue, 25 Jan 2022 & \textbf{  Prob (F-statistic):} &  2.41e-11   \\
\textbf{Time:}             &     02:33:02     & \textbf{  Log-Likelihood:    } &    2838.6   \\
\textbf{No. Observations:} &        3072      & \textbf{  AIC:               } &    -5673.   \\
\textbf{Df Residuals:}     &        3070      & \textbf{  BIC:               } &    -5661.   \\
\textbf{Df Model:}         &           1      & \textbf{                     } &             \\
\bottomrule
\end{tabular}
\begin{tabular}{lcccccc}
                     & \textbf{coef} & \textbf{std err} & \textbf{t} & \textbf{P$> |$t$|$} & \textbf{[0.025} & \textbf{0.975]}  \\
\midrule
\textbf{Intercept}   &       0.5168  &        0.009     &    57.201  &         0.000        &        0.499    &        0.535     \\
\textbf{white\_perc} &      -0.0712  &        0.011     &    -6.704  &         0.000        &       -0.092    &       -0.050     \\
\bottomrule
\end{tabular}
\begin{tabular}{lclc}
\textbf{Omnibus:}       & 493.539 & \textbf{  Durbin-Watson:     } &    1.881  \\
\textbf{Prob(Omnibus):} &   0.000 & \textbf{  Jarque-Bera (JB):  } & 8149.340  \\
\textbf{Skew:}          &  -0.183 & \textbf{  Prob(JB):          } &     0.00  \\
\textbf{Kurtosis:}      &  10.971 & \textbf{  Cond. No.          } &     10.5  \\
\bottomrule
\end{tabular}
%\caption{OLS Regression Results}
\end{center}

\section{coeff}

 black_perc weighted
\begin{center}
\begin{tabular}{lclc}
\toprule
\textbf{Dep. Variable:}    &  promoted\_perc  & \textbf{  R-squared:         } &      0.008    \\
\textbf{Model:}            &       WLS        & \textbf{  Adj. R-squared:    } &      0.008    \\
\textbf{Method:}           &  Least Squares   & \textbf{  F-statistic:       } &      25.78    \\
\textbf{Date:}             & Thu, 24 Feb 2022 & \textbf{  Prob (F-statistic):} &   4.06e-07    \\
\textbf{Time:}             &     23:26:46     & \textbf{  Log-Likelihood:    } &    -718.34    \\
\textbf{No. Observations:} &        3099      & \textbf{  AIC:               } &      1441.    \\
\textbf{Df Residuals:}     &        3097      & \textbf{  BIC:               } &      1453.    \\
\textbf{Df Model:}         &           1      & \textbf{                     } &               \\
\bottomrule
\end{tabular}
\begin{tabular}{lcccccc}
                     & \textbf{coef} & \textbf{std err} & \textbf{t} & \textbf{P$> |$t$|$} & \textbf{[0.025} & \textbf{0.975]}  \\
\midrule
\textbf{const}       &       0.4919  &        0.002     &   245.644  &         0.000        &        0.488    &        0.496     \\
\textbf{black\_perc} &       0.0524  &        0.010     &     5.077  &         0.000        &        0.032    &        0.073     \\
\bottomrule
\end{tabular}
\begin{tabular}{lclc}
\textbf{Omnibus:}       & 2724.328 & \textbf{  Durbin-Watson:     } &      1.995    \\
\textbf{Prob(Omnibus):} &   0.000  & \textbf{  Jarque-Bera (JB):  } & 13207561.210  \\
\textbf{Skew:}          &  -2.624  & \textbf{  Prob(JB):          } &       0.00    \\
\textbf{Kurtosis:}      & 322.777  & \textbf{  Cond. No.          } &       8.09    \\
\bottomrule
\end{tabular}
%\caption{WLS Regression Results}
\end{center}

Warnings: \newline
 [1] Standard Errors assume that the covariance matrix of the errors is correctly specified.

 black_perc unweighted
\begin{center}
\begin{tabular}{lclc}
\toprule
\textbf{Dep. Variable:}    &  promoted\_perc  & \textbf{  R-squared:         } &     0.008   \\
\textbf{Model:}            &       OLS        & \textbf{  Adj. R-squared:    } &     0.007   \\
\textbf{Method:}           &  Least Squares   & \textbf{  F-statistic:       } &     24.29   \\
\textbf{Date:}             & Thu, 24 Feb 2022 & \textbf{  Prob (F-statistic):} &  8.70e-07   \\
\textbf{Time:}             &     23:26:46     & \textbf{  Log-Likelihood:    } &    2843.6   \\
\textbf{No. Observations:} &        3099      & \textbf{  AIC:               } &    -5683.   \\
\textbf{Df Residuals:}     &        3097      & \textbf{  BIC:               } &    -5671.   \\
\textbf{Df Model:}         &           1      & \textbf{                     } &             \\
\bottomrule
\end{tabular}
\begin{tabular}{lcccccc}
                     & \textbf{coef} & \textbf{std err} & \textbf{t} & \textbf{P$> |$t$|$} & \textbf{[0.025} & \textbf{0.975]}  \\
\midrule
\textbf{Intercept}   &       0.4520  &        0.002     &   220.889  &         0.000        &        0.448    &        0.456     \\
\textbf{black\_perc} &       0.0593  &        0.012     &     4.929  &         0.000        &        0.036    &        0.083     \\
\bottomrule
\end{tabular}
\begin{tabular}{lclc}
\textbf{Omnibus:}       & 499.817 & \textbf{  Durbin-Watson:     } &    1.887  \\
\textbf{Prob(Omnibus):} &   0.000 & \textbf{  Jarque-Bera (JB):  } & 7874.859  \\
\textbf{Skew:}          &  -0.226 & \textbf{  Prob(JB):          } &     0.00  \\
\textbf{Kurtosis:}      &  10.796 & \textbf{  Cond. No.          } &     6.98  \\
\bottomrule
\end{tabular}
%\caption{OLS Regression Results}
\end{center}

Warnings: \newline
 [1] Standard Errors assume that the covariance matrix of the errors is correctly specified.

 white_perc weighted
\begin{center}
\begin{tabular}{lclc}
\toprule
\textbf{Dep. Variable:}    &  promoted\_perc  & \textbf{  R-squared:         } &      0.095    \\
\textbf{Model:}            &       WLS        & \textbf{  Adj. R-squared:    } &      0.095    \\
\textbf{Method:}           &  Least Squares   & \textbf{  F-statistic:       } &      326.3    \\
\textbf{Date:}             & Thu, 24 Feb 2022 & \textbf{  Prob (F-statistic):} &   1.98e-69    \\
\textbf{Time:}             &     23:26:46     & \textbf{  Log-Likelihood:    } &    -575.96    \\
\textbf{No. Observations:} &        3099      & \textbf{  AIC:               } &      1156.    \\
\textbf{Df Residuals:}     &        3097      & \textbf{  BIC:               } &      1168.    \\
\textbf{Df Model:}         &           1      & \textbf{                     } &               \\
\bottomrule
\end{tabular}
\begin{tabular}{lcccccc}
                     & \textbf{coef} & \textbf{std err} & \textbf{t} & \textbf{P$> |$t$|$} & \textbf{[0.025} & \textbf{0.975]}  \\
\midrule
\textbf{const}       &       0.5940  &        0.005     &   110.703  &         0.000        &        0.583    &        0.604     \\
\textbf{white\_perc} &      -0.1451  &        0.008     &   -18.064  &         0.000        &       -0.161    &       -0.129     \\
\bottomrule
\end{tabular}
\begin{tabular}{lclc}
\textbf{Omnibus:}       & 3501.718 & \textbf{  Durbin-Watson:     } &      2.042    \\
\textbf{Prob(Omnibus):} &   0.000  & \textbf{  Jarque-Bera (JB):  } & 10847867.277  \\
\textbf{Skew:}          &  -4.537  & \textbf{  Prob(JB):          } &       0.00    \\
\textbf{Kurtosis:}      & 292.704  & \textbf{  Cond. No.          } &       9.23    \\
\bottomrule
\end{tabular}
%\caption{WLS Regression Results}
\end{center}

Warnings: \newline
 [1] Standard Errors assume that the covariance matrix of the errors is correctly specified.

 white_perc unweighted
\begin{center}
\begin{tabular}{lclc}
\toprule
\textbf{Dep. Variable:}    &  promoted\_perc  & \textbf{  R-squared:         } &     0.013   \\
\textbf{Model:}            &       OLS        & \textbf{  Adj. R-squared:    } &     0.012   \\
\textbf{Method:}           &  Least Squares   & \textbf{  F-statistic:       } &     39.88   \\
\textbf{Date:}             & Thu, 24 Feb 2022 & \textbf{  Prob (F-statistic):} &  3.09e-10   \\
\textbf{Time:}             &     23:26:46     & \textbf{  Log-Likelihood:    } &    2851.3   \\
\textbf{No. Observations:} &        3099      & \textbf{  AIC:               } &    -5699.   \\
\textbf{Df Residuals:}     &        3097      & \textbf{  BIC:               } &    -5687.   \\
\textbf{Df Model:}         &           1      & \textbf{                     } &             \\
\bottomrule
\end{tabular}
\begin{tabular}{lcccccc}
                     & \textbf{coef} & \textbf{std err} & \textbf{t} & \textbf{P$> |$t$|$} & \textbf{[0.025} & \textbf{0.975]}  \\
\midrule
\textbf{Intercept}   &       0.5116  &        0.009     &    58.266  &         0.000        &        0.494    &        0.529     \\
\textbf{white\_perc} &      -0.0654  &        0.010     &    -6.315  &         0.000        &       -0.086    &       -0.045     \\
\bottomrule
\end{tabular}
\begin{tabular}{lclc}
\textbf{Omnibus:}       & 503.711 & \textbf{  Durbin-Watson:     } &    1.888  \\
\textbf{Prob(Omnibus):} &   0.000 & \textbf{  Jarque-Bera (JB):  } & 8153.276  \\
\textbf{Skew:}          &  -0.219 & \textbf{  Prob(JB):          } &     0.00  \\
\textbf{Kurtosis:}      &  10.934 & \textbf{  Cond. No.          } &     10.2  \\
\bottomrule
\end{tabular}
%\caption{OLS Regression Results}
\end{center}

Warnings: \newline
 [1] Standard Errors assume that the covariance matrix of the errors is correctly specified.

 not_hispanic_or_latino_white_only_perc weighted
\begin{center}
\begin{tabular}{lclc}
\toprule
\textbf{Dep. Variable:}                               &  promoted\_perc  & \textbf{  R-squared:         } &      0.111    \\
\textbf{Model:}                                       &       WLS        & \textbf{  Adj. R-squared:    } &      0.111    \\
\textbf{Method:}                                      &  Least Squares   & \textbf{  F-statistic:       } &      388.5    \\
\textbf{Date:}                                        & Thu, 24 Feb 2022 & \textbf{  Prob (F-statistic):} &   1.43e-81    \\
\textbf{Time:}                                        &     23:26:46     & \textbf{  Log-Likelihood:    } &    -548.06    \\
\textbf{No. Observations:}                            &        3099      & \textbf{  AIC:               } &      1100.    \\
\textbf{Df Residuals:}                                &        3097      & \textbf{  BIC:               } &      1112.    \\
\textbf{Df Model:}                                    &           1      & \textbf{                     } &               \\
\bottomrule
\end{tabular}
\begin{tabular}{lcccccc}
                                                      & \textbf{coef} & \textbf{std err} & \textbf{t} & \textbf{P$> |$t$|$} & \textbf{[0.025} & \textbf{0.975]}  \\
\midrule
\textbf{const}                                        &       0.5625  &        0.003     &   164.628  &         0.000        &        0.556    &        0.569     \\
\textbf{not\_hispanic\_or\_latino\_white\_only\_perc} &      -0.1223  &        0.006     &   -19.711  &         0.000        &       -0.135    &       -0.110     \\
\bottomrule
\end{tabular}
\begin{tabular}{lclc}
\textbf{Omnibus:}       & 3512.706 & \textbf{  Durbin-Watson:     } &      2.062    \\
\textbf{Prob(Omnibus):} &   0.000  & \textbf{  Jarque-Bera (JB):  } & 12337552.519  \\
\textbf{Skew:}          &  -4.533  & \textbf{  Prob(JB):          } &       0.00    \\
\textbf{Kurtosis:}      & 311.974  & \textbf{  Cond. No.          } &       6.41    \\
\bottomrule
\end{tabular}
%\caption{WLS Regression Results}
\end{center}

Warnings: \newline
 [1] Standard Errors assume that the covariance matrix of the errors is correctly specified.

 not_hispanic_or_latino_white_only_perc unweighted
\begin{center}
\begin{tabular}{lclc}
\toprule
\textbf{Dep. Variable:}                               &  promoted\_perc  & \textbf{  R-squared:         } &     0.029   \\
\textbf{Model:}                                       &       OLS        & \textbf{  Adj. R-squared:    } &     0.029   \\
\textbf{Method:}                                      &  Least Squares   & \textbf{  F-statistic:       } &     93.11   \\
\textbf{Date:}                                        & Thu, 24 Feb 2022 & \textbf{  Prob (F-statistic):} &  9.99e-22   \\
\textbf{Time:}                                        &     23:26:46     & \textbf{  Log-Likelihood:    } &    2877.4   \\
\textbf{No. Observations:}                            &        3099      & \textbf{  AIC:               } &    -5751.   \\
\textbf{Df Residuals:}                                &        3097      & \textbf{  BIC:               } &    -5739.   \\
\textbf{Df Model:}                                    &           1      & \textbf{                     } &             \\
\bottomrule
\end{tabular}
\begin{tabular}{lcccccc}
                                                      & \textbf{coef} & \textbf{std err} & \textbf{t} & \textbf{P$> |$t$|$} & \textbf{[0.025} & \textbf{0.975]}  \\
\midrule
\textbf{Intercept}                                    &       0.5205  &        0.007     &    76.835  &         0.000        &        0.507    &        0.534     \\
\textbf{not\_hispanic\_or\_latino\_white\_only\_perc} &      -0.0825  &        0.009     &    -9.649  &         0.000        &       -0.099    &       -0.066     \\
\bottomrule
\end{tabular}
\begin{tabular}{lclc}
\textbf{Omnibus:}       & 523.874 & \textbf{  Durbin-Watson:     } &    1.898  \\
\textbf{Prob(Omnibus):} &   0.000 & \textbf{  Jarque-Bera (JB):  } & 8945.658  \\
\textbf{Skew:}          &  -0.246 & \textbf{  Prob(JB):          } &     0.00  \\
\textbf{Kurtosis:}      &  11.309 & \textbf{  Cond. No.          } &     7.98  \\
\bottomrule
\end{tabular}
%\caption{OLS Regression Results}
\end{center}

Warnings: \newline
 [1] Standard Errors assume that the covariance matrix of the errors is correctly specified.

 not_hispanic_or_latino_black_only_perc weighted
\begin{center}
\begin{tabular}{lclc}
\toprule
\textbf{Dep. Variable:}                               &  promoted\_perc  & \textbf{  R-squared:         } &      0.009    \\
\textbf{Model:}                                       &       WLS        & \textbf{  Adj. R-squared:    } &      0.009    \\
\textbf{Method:}                                      &  Least Squares   & \textbf{  F-statistic:       } &      28.76    \\
\textbf{Date:}                                        & Thu, 24 Feb 2022 & \textbf{  Prob (F-statistic):} &   8.79e-08    \\
\textbf{Time:}                                        &     23:26:46     & \textbf{  Log-Likelihood:    } &    -716.86    \\
\textbf{No. Observations:}                            &        3099      & \textbf{  AIC:               } &      1438.    \\
\textbf{Df Residuals:}                                &        3097      & \textbf{  BIC:               } &      1450.    \\
\textbf{Df Model:}                                    &           1      & \textbf{                     } &               \\
\bottomrule
\end{tabular}
\begin{tabular}{lcccccc}
                                                      & \textbf{coef} & \textbf{std err} & \textbf{t} & \textbf{P$> |$t$|$} & \textbf{[0.025} & \textbf{0.975]}  \\
\midrule
\textbf{const}                                        &       0.4918  &        0.002     &   250.017  &         0.000        &        0.488    &        0.496     \\
\textbf{not\_hispanic\_or\_latino\_black\_only\_perc} &       0.0560  &        0.010     &     5.363  &         0.000        &        0.036    &        0.076     \\
\bottomrule
\end{tabular}
\begin{tabular}{lclc}
\textbf{Omnibus:}       & 2705.140 & \textbf{  Durbin-Watson:     } &      1.995    \\
\textbf{Prob(Omnibus):} &   0.000  & \textbf{  Jarque-Bera (JB):  } & 13255122.492  \\
\textbf{Skew:}          &  -2.583  & \textbf{  Prob(JB):          } &       0.00    \\
\textbf{Kurtosis:}      & 323.354  & \textbf{  Cond. No.          } &       8.19    \\
\bottomrule
\end{tabular}
%\caption{WLS Regression Results}
\end{center}

Warnings: \newline
 [1] Standard Errors assume that the covariance matrix of the errors is correctly specified.

 not_hispanic_or_latino_black_only_perc unweighted
\begin{center}
\begin{tabular}{lclc}
\toprule
\textbf{Dep. Variable:}                               &  promoted\_perc  & \textbf{  R-squared:         } &     0.008   \\
\textbf{Model:}                                       &       OLS        & \textbf{  Adj. R-squared:    } &     0.007   \\
\textbf{Method:}                                      &  Least Squares   & \textbf{  F-statistic:       } &     23.58   \\
\textbf{Date:}                                        & Thu, 24 Feb 2022 & \textbf{  Prob (F-statistic):} &  1.25e-06   \\
\textbf{Time:}                                        &     23:26:46     & \textbf{  Log-Likelihood:    } &    2843.3   \\
\textbf{No. Observations:}                            &        3099      & \textbf{  AIC:               } &    -5683.   \\
\textbf{Df Residuals:}                                &        3097      & \textbf{  BIC:               } &    -5670.   \\
\textbf{Df Model:}                                    &           1      & \textbf{                     } &             \\
\bottomrule
\end{tabular}
\begin{tabular}{lcccccc}
                                                      & \textbf{coef} & \textbf{std err} & \textbf{t} & \textbf{P$> |$t$|$} & \textbf{[0.025} & \textbf{0.975]}  \\
\midrule
\textbf{Intercept}                                    &       0.4521  &        0.002     &   221.591  &         0.000        &        0.448    &        0.456     \\
\textbf{not\_hispanic\_or\_latino\_black\_only\_perc} &       0.0587  &        0.012     &     4.856  &         0.000        &        0.035    &        0.082     \\
\bottomrule
\end{tabular}
\begin{tabular}{lclc}
\textbf{Omnibus:}       & 499.771 & \textbf{  Durbin-Watson:     } &    1.887  \\
\textbf{Prob(Omnibus):} &   0.000 & \textbf{  Jarque-Bera (JB):  } & 7866.672  \\
\textbf{Skew:}          &  -0.226 & \textbf{  Prob(JB):          } &     0.00  \\
\textbf{Kurtosis:}      &  10.792 & \textbf{  Cond. No.          } &     7.01  \\
\bottomrule
\end{tabular}
%\caption{OLS Regression Results}
\end{center}
